# Supplementary material for: QHackBench: Benchmarking Large Language Models for Quantum Code Generation Using PennyLane Hackathon Challenges
Source: arXiv:2506.20008 source file (2025-08-29)
Supplement: Supplementary file 1 [file appendix.tex]

\section*{Apendix}

\begin{table}[htbp]
\centering
\caption{Pass@k Results for 2023 Challenges (\textbf{4o-mini} and \textbf{o3-mini})}
\label{tab:passk2023}
\begin{adjustbox}{max width=1\linewidth}
\begin{tabular}{lrrrr}
\toprule
Challenge                      & \textbf{4o-mini RAG Pass Rate (\%)} & \textbf{4o-mini Non-RAG Pass Rate (\%)} & \textbf{o3-mini RAG Pass Rate (\%)} & \textbf{o3-mini Non-RAG Pass Rate (\%)} \\
\midrule
/tutorial\_6                 & 100.00  & 66.67  & 100.00  & 100.00  \\
/tutorial\_1                 & 100.00  & 100.00  & 100.00  & 100.00  \\
/tutorial\_5                 & 0.00    & 0.00    & 0.00    & 0.00    \\
/tutorial\_4                 & 0.00    & 0.00    & 100.00  & 100.00  \\
/tutorial\_3                 & 0.00    & 0.00    & 0.00    & 0.00    \\
/tutorial\_7                 & 0.00    & 0.00    & 0.00    & 0.00    \\
/tutorial\_2                 & 100.00  & 0.00    & 100.00  & 100.00  \\
/tutorial\_8                 & 0.00    & 0.00    & 0.00    & 0.00    \\
a\_tale\_of\_timbits\_100    & 0.00    & 0.00    & 0.00    & 0.00    \\
a\_tale\_of\_timbits\_200    & 0.00    & 0.00    & 0.00    & 0.00    \\
a\_tale\_of\_timbits\_500    & 0.00    & 0.00    & 0.00    & 0.00    \\
a\_tale\_of\_timbits\_400    & 0.00    & 0.00    & 33.33   & 0.00    \\
a\_tale\_of\_timbits\_300    & 0.00    & 0.00    & 0.00    & 33.33   \\
fall\_of\_sqynet\_200        & 0.00    & 0.00    & 66.67   & 100.00  \\
fall\_of\_sqynet\_300        & 0.00    & 0.00    & 0.00    & 100.00  \\
fall\_of\_sqynet\_100        & 0.00    & 0.00    & 0.00    & 0.00    \\
fall\_of\_sqynet\_400        & 0.00    & 0.00    & 0.00    & 66.67   \\
fall\_of\_sqynet\_500        & 66.67   & 33.33   & 66.67   & 0.00    \\
office\_hijinks\_300         & 100.00  & 66.67   & 100.00  & 0.00    \\
office\_hijinks\_500         & 0.00    & 0.00    & 0.00    & 0.00    \\
office\_hijinks\_100         & 100.00  & 66.67   & 100.00  & 100.00  \\
office\_hijinks\_200         & 0.00    & 0.00    & 0.00    & 33.33   \\
office\_hijinks\_400         & 0.00    & 0.00    & 0.00    & 0.00    \\
bending\_bennets\_laws\_400  & 0.00    & 33.33   & 100.00  & 100.00  \\
bending\_bennets\_laws\_500  & 0.00    & 0.00    & 0.00    & 33.33   \\
bending\_bennets\_laws\_100  & 100.00  & 100.00  & 100.00  & 100.00  \\
bending\_bennets\_laws\_300  & 0.00    & 0.00    & 0.00    & 100.00  \\
bending\_bennets\_laws\_200  & 0.00    & 0.00    & 0.00    & 66.67   \\
\bottomrule
\end{tabular}
\end{adjustbox}
\end{table}

\begin{table}[htbp]
\centering
\caption{Pass@k Results for 2024 Challenges}
\label{tab:passk2024}
\begin{adjustbox}{max width=1\linewidth}
\begin{tabular}{lrr}
\toprule
Challenge                & RAG Pass Rate (\%) & Non-RAG Pass Rate (\%) \\
\midrule
GHZ\_inn                 & 100.0              & 33.33                \\
rainy\_days\_retreat     & 100.0              & 100.0                \\
wormhole\_airdrome       & 0.0                & 0.0                  \\
mach\_zender\_cabin      & 33.33              & 0.0                  \\
chalet\_random\_gate     & 0.0                & 0.0                  \\
save\_qhack\_beach       & 0.0                & 0.0                  \\
market\_quantum\_trinkets& 0.0                & 0.0                  \\
travelling\_eigentracks  & 0.0                & 0.0                  \\
ruins\_oasis             & 0.0                & 0.0                  \\
hacking\_for\_upgrayde    & 100.0              & 100.0                \\
QSP\_swamp               & 100.0              & 100.0                \\
triple\_H\_hotel         & 0.0                & 0.0                  \\
fireworks\_qutropolis    & 0.0                & 0.0                  \\
lazy\_workers\_terminal   & 0.0                & 0.0                  \\
hockey\_night\_cave      & 0.0                & 0.0                  \\
to\_view\_or\_not\_to\_view& 100.0              & 100.0                \\
mojito\_hhlime\_twist    & 0.0                & 0.0                  \\
coffee\_conundrum        & 0.0                & 0.0                  \\
contextuality\_dunes     & 0.0                & 33.33                \\
mathematicians\_at\_resort& 0.0                & 33.33                \\
three\_shipping\_companies& 0.0                & 0.0                  \\
\bottomrule
\end{tabular}
\end{adjustbox}
\end{table}

\begin{table}[htbp]
\centering
\tiny
\caption{Pass@k Results for 2023 Challenges (\textbf{o3-mini and 4o-mini})}
\label{tab:passk2023}
\begin{adjustbox}{max width=1\linewidth}
\begin{tabular}{lrrrr}

\toprule
Challenge                      & \textbf{\makecell{o3-mini\\ RAG\\ Pass Rate\\ (\%)}} & \textbf{\makecell{o3-mini\\ Non-RAG\\ Pass Rate\\ (\%)}} & \textbf{\makecell{4o-mini\\ RAG\\ Pass Rate\\ (\%)}} & \textbf{\makecell{4o-mini\\ Non-RAG\\ Pass Rate\\ (\%)}} \\
\midrule
C6-E-23 & 100.00  & 100.00  & 100.00  & 66.67  \\
C1-E-23 & 100.00  & 100.00  & 100.00  & 100.00  \\
C5-E-23 & 0.00    & 0.00    & 0.00    & 0.00    \\
C4-E-23 & 100.00  & 100.00  & 0.00    & 0.00    \\
C3-E-23 & 0.00    & 0.00    & 0.00    & 0.00    \\
C7-E-23 & 0.00    & 0.00    & 0.00    & 0.00    \\
C2-E-23 & 100.00  & 100.00  & 100.00  & 0.00    \\
C8-E-23 & 0.00    & 0.00    & 0.00    & 0.00    \\
C9-E-23 & 0.00    & 0.00    & 0.00    & 0.00    \\
C10-I-23 & 0.00    & 0.00    & 0.00    & 0.00    \\
C13-A-23 & 0.00    & 0.00    & 0.00    & 0.00    \\
C12-A-23 & 33.33   & 0.00    & 0.00    & 0.00    \\
C11-I-23 & 0.00    & 33.33   & 0.00    & 0.00    \\
C20-I-23 & 66.67   & 100.00  & 0.00    & 0.00    \\
C21-I-23 & 0.00    & 100.00  & 0.00    & 0.00    \\
C19-E-23 & 0.00    & 0.00    & 0.00    & 0.00    \\
C22-A-23 & 0.00    & 66.67   & 0.00    & 0.00    \\
C23-A-23 & 66.67   & 0.00    & 66.67   & 33.33   \\
C26-I-23 & 100.00  & 0.00    & 100.00  & 66.67   \\
C28-A-23 & 0.00    & 0.00    & 0.00    & 0.00    \\
C24-E-23 & 100.00  & 100.00  & 100.00  & 66.67   \\
C25-I-23 & 0.00    & 33.33   & 0.00    & 0.00    \\
C27-A-23 & 0.00    & 0.00    & 0.00    & 0.00    \\
C17-A-23 & 100.00  & 100.00  & 0.00    & 33.33   \\
C18-A-23 & 0.00    & 33.33   & 0.00    & 0.00    \\
C14-E-23 & 100.00  & 100.00  & 100.00  & 100.00  \\
C15-I-23 & 0.00    & 100.00  & 0.00    & 0.00    \\
C16-I-23 & 0.00    & 66.67   & 0.00    & 0.00    \\
\bottomrule
\end{tabular}
\end{adjustbox}
\end{table}
